# Supplementary material for: Physics-Inspired Heuristics for Soft MIMO Detection in 5G New Radio and Beyond
Source: arXiv:2103.10561 source file (2021-03-18)
Supplement: Supplementary file 1 [file timing_appendix.tex]

\section{Timing the PMIS} 
Each PMIS run has slightly different runtimes, which is not a desirable system property, since it causes overall latency increase and hardware synchronization issues. 
%To solve this, a PMIS \emph{timer} is used to rule out some outliers by setting a time out period as 99.5th percentile of runtimes out of 250,000 test PMIS runs per MIMO size and modulation. This implies that \systemname{} can achieve the consistent latency but $N_{PE}$ is not exactly the number of collected PMIS outputs; PMIS runs on $N_{PE}+\alpha$ processing elements can lead to $N_{PE}$ PMIS outputs, where $\alpha=\frac{5}{995}N_{PE}$. 
{\DV{In the benchmarking procedure, we neglect variations in latency of different PEs, reporting the runtime as the $99.5\%$ percentile of the measured runtimes, for each instance, and we discard the corresponding fraction of $0.05\%$ anomalously slow processes.}}
%assume PMIS runs on $N_{PE}$ processing elements yeild $N_{PE}$ PMIS outputs for the rest of the paper{\DV{, even if we ignore the 5\% slowest }}. 
%(\emph{i.e}, ignoring $\alpha$), since $\alpha$ is relatively small (1 per {\it ca.} 200 $N_{PE}$) and can be considered afterwards when necessary.
Note that the runtime variation can be reduced by an integrated system hardware since 
%most of the outliers are reported 
{\DV{the origin of the variations is}}
caused by the randomness introduced by the Metropolis updated (which can be eventually ``de-randomized'') and the 
overlapping operating system usage {\DV{by different processes not related to our benchmarking.}}
%and adjustable timeout duration is also available considering environments. %(\emph{e.g.}, if $N_{PE}$ are enough, timeout length becomes shorter value such as 75th. runtime).

In the detailed view in Figure~\ref{f:sweep_opt} (\emph{right, top}), it is shown that most of the runtimes are below 350~$\mu$s while some outliers are over 400~$\mu$s. 
% The upper whiskers of the box plots are pointing out the 99.5th percentile and 
As mentioned in the design section, the mean value of 99.5th percentile of runtimes is used for the PMIS timer. Note that the gap between median runtime and 99.5th percentile is only 20-30 $\mu$s and this variation can be further reduced on the integrated hardware. Figure~\ref{f:compute_vs_nv} shows the computing time of \systemname{} across the numbers of variables $N_V$ per channel use. As the number of variables increases (\emph{i.e.}, MIMO size and/or modulation increases), computing time tends to increase, where $N_V=160$ reaches the approximate borderline of the LTE standards. The available largest MIMO size in terms of the compute time for the LTE is 160, 80, 40 for BPSK, QPSK, 16-QAM modulation, respectively. Recall that available processing time in the LTE is at most 3~ms including error channel coding.
